# Supplementary material for: ColorSense: A Study on Color Vision in Machine Visual Recognition
Source: arXiv:2212.08650 source file (2025-02-13)
Supplement: Supplementary file 2 [file supp_tab_cifar100-f.tex]

\begin{table*}[h]
\centering
  \begin{adjustbox}{max width=\textwidth}
   \begin{tabular}{lcccccccc}
    \toprule
    Classes & Green & Gray & Blue & White & Black & Brown & Red & Others  \\
    
     \midrule
    streetcar & 21 & 2 & 6 & 5 & 3 & 19 & 38 & 6 \\
    apple & 6 & 0 & 0 & 0 & 0 & 9 & 69 & 16 \\
    palm_tree & 95 & 0 & 0 & 0 & 1 & 1 & 0 & 3 \\
    man & 0 & 0 & 0 & 72 & 6 & 5 & 0 & 17 \\
    forest & 53 & 0 & 0 & 0 & 9 & 26 & 1 & 11 \\
    butterfly & 3 & 1 & 6 & 5 & 14 & 58 & 10 & 3 \\
    lamp & 3 & 4 & 8 & 16 & 26 & 32 & 4 & 7 \\
    wardrobe & 0 & 3 & 0 & 13 & 0 & 81 & 2 & 1 \\
    pear & 37 & 1 & 0 & 4 & 0 & 46 & 6 & 6 \\
    raccoon & 0 & 6 & 0 & 5 & 4 & 84 & 1 & 0 \\
    crab & 8 & 2 & 0 & 0 & 9 & 15 & 51 & 15 \\
    tractor & 8 & 1 & 6 & 0 & 0 & 72 & 12 & 1 \\
    aquarium_fish & 0 & 2 & 20 & 3 & 0 & 21 & 28 & 26 \\
    can & 12 & 11 & 10 & 18 & 3 & 11 & 16 & 19 \\
    tank & 55 & 14 & 1 & 0 & 12 & 15 & 0 & 3 \\
    snail & 6 & 6 & 1 & 10 & 0 & 71 & 2 & 4 \\
    bed & 0 & 5 & 11 & 42 & 1 & 16 & 8 & 17 \\
    cup & 10 & 9 & 8 & 14 & 6 & 24 & 3 & 26 \\
    television & 0 & 37 & 3 & 9 & 43 & 7 & 1 & 0 \\
    turtle & 29 & 5 & 13 & 3 & 10 & 33 & 0 & 7 \\
    boy & 0 & 0 & 0 & 72 & 18 & 4 & 0 & 6 \\
    mushroom & 1 & 0 & 0 & 26 & 0 & 65 & 5 & 3 \\
    bee & 0 & 0 & 0 & 1 & 32 & 64 & 0 & 3 \\
    fox & 0 & 0 & 0 & 7 & 0 & 93 & 0 & 0 \\
    willow_tree & 78 & 3 & 2 & 0 & 0 & 12 & 3 & 2 \\
    couch & 8 & 4 & 11 & 22 & 10 & 29 & 7 & 9 \\
    dolphin & 5 & 53 & 19 & 1 & 18 & 4 & 0 & 0 \\
    cattle & 0 & 0 & 0 & 13 & 24 & 55 & 0 & 8 \\
    maple_tree & 58 & 0 & 0 & 1 & 5 & 8 & 24 & 4 \\
    plain & 53 & 2 & 3 & 1 & 2 & 38 & 1 & 0 \\
    bear & 0 & 0 & 0 & 20 & 30 & 49 & 0 & 1 \\
    bridge & 5 & 36 & 1 & 9 & 18 & 20 & 6 & 5 \\
    leopard & 2 & 6 & 0 & 11 & 2 & 77 & 0 & 2 \\
    hamster & 1 & 2 & 0 & 23 & 0 & 74 & 0 & 0 \\
    lawn_mower & 26 & 2 & 0 & 0 & 15 & 8 & 35 & 14 \\
    lobster & 12 & 1 & 8 & 3 & 9 & 20 & 37 & 10 \\
    camel & 0 & 0 & 0 & 17 & 7 & 74 & 0 & 2 \\
    tiger & 0 & 0 & 0 & 3 & 0 & 96 & 0 & 1 \\
    road & 2 & 38 & 0 & 3 & 43 & 14 & 0 & 0 \\
    whale & 0 & 23 & 14 & 7 & 54 & 2 & 0 & 0 \\
    motorcycle & 5 & 0 & 21 & 6 & 19 & 13 & 25 & 11 \\
    crocodile & 50 & 1 & 4 & 4 & 10 & 29 & 1 & 1 \\
    dinosaur & 37 & 2 & 7 & 1 & 2 & 40 & 4 & 7 \\
    chair & 6 & 5 & 11 & 8 & 8 & 49 & 10 & 3 \\
    bus & 7 & 6 & 11 & 30 & 1 & 24 & 13 & 8 \\
    plate & 8 & 1 & 13 & 34 & 1 & 11 & 1 & 31 \\
    otter & 6 & 3 & 0 & 11 & 6 & 74 & 0 & 0 \\
    rose & 0 & 0 & 1 & 7 & 0 & 10 & 80 & 2 \\
    seal & 4 & 4 & 5 & 19 & 8 & 56 & 0 & 4 \\
    telephone & 1 & 7 & 11 & 23 & 50 & 7 & 1 & 0 \\
    mouse & 3 & 16 & 0 & 11 & 5 & 62 & 2 & 1 \\
    \bottomrule
  \end{tabular}
  \end{adjustbox}
  \caption{\textbf{CIFAR100-F Statistics (part 1).} The number of instances that belongs to each foreground color from each class.}
  \label{tab:cifar100b_appendix}
\end{table*}

\begin{table*}[h]
\centering
  \begin{adjustbox}{max width=\textwidth}
   \begin{tabular}{lcccccccc}
    \toprule
    Classes & Green & Gray & Blue & White & Black & Brown & Red & Others  \\
     \midrule
        
    tulip & 0 & 0 & 5 & 12 & 0 & 22 & 61 & 0 \\
    porcupine & 0 & 4 & 0 & 1 & 8 & 85 & 0 & 2 \\
    beaver & 0 & 7 & 0 & 0 & 10 & 82 & 0 & 1 \\
    wolf & 0 & 31 & 0 & 17 & 4 & 48 & 0 & 0 \\
    lizard & 37 & 7 & 3 & 1 & 0 & 32 & 2 & 18 \\
    flatfish & 10 & 5 & 2 & 22 & 5 & 52 & 1 & 3 \\
    beetle & 30 & 2 & 7 & 0 & 18 & 13 & 22 & 8 \\
    chimpanzee & 0 & 7 & 0 & 1 & 59 & 33 & 0 & 0 \\
    poppy & 0 & 0 & 3 & 3 & 0 & 35 & 56 & 3 \\
    bowl & 10 & 0 & 8 & 17 & 4 & 19 & 7 & 35 \\
    table & 6 & 4 & 3 & 25 & 0 & 58 & 2 & 2 \\
    shrew & 0 & 3 & 0 & 2 & 18 & 77 & 0 & 0 \\
    skyscraper & 6 & 33 & 44 & 0 & 9 & 8 & 0 & 0 \\
    kangaroo & 0 & 3 & 0 & 9 & 7 & 81 & 0 & 0 \\
    cloud & 0 & 5 & 7 & 74 & 6 & 1 & 5 & 2 \\
    girl & 0 & 0 & 0 & 79 & 11 & 10 & 0 & 0 \\
    worm & 18 & 6 & 16 & 4 & 10 & 32 & 11 & 3 \\
    train & 13 & 7 & 13 & 0 & 10 & 23 & 15 & 19 \\
    house & 6 & 4 & 6 & 27 & 0 & 35 & 3 & 19 \\
    caterpillar & 45 & 0 & 1 & 6 & 8 & 10 & 8 & 22 \\
    spider & 6 & 0 & 3 & 5 & 19 & 34 & 0 & 33 \\
    rabbit & 0 & 4 & 0 & 33 & 10 & 52 & 0 & 1 \\
    cockroach & 2 & 0 & 2 & 0 & 32 & 58 & 3 & 3 \\
    rocket & 11 & 10 & 2 & 43 & 20 & 7 & 1 & 6 \\
    castle & 0 & 22 & 1 & 32 & 0 & 42 & 1 & 2 \\
    bicycle & 10 & 10 & 11 & 5 & 27 & 4 & 13 & 20 \\
    baby & 0 & 0 & 0 & 63 & 8 & 7 & 16 & 6 \\
    mountain & 15 & 10 & 7 & 43 & 2 & 19 & 1 & 3 \\
    sweet_pepper & 29 & 0 & 0 & 0 & 0 & 27 & 25 & 19 \\
    orchid & 5 & 0 & 1 & 31 & 0 & 7 & 53 & 3 \\
    sea & 2 & 12 & 64 & 5 & 7 & 2 & 0 & 8 \\
    skunk & 0 & 0 & 0 & 1 & 79 & 19 & 0 & 1 \\
    oak_tree & 96 & 0 & 0 & 0 & 2 & 2 & 0 & 0 \\
    squirrel & 1 & 12 & 0 & 2 & 7 & 78 & 0 & 0 \\
    ray & 10 & 23 & 21 & 9 & 14 & 12 & 1 & 10 \\
    bottle & 19 & 1 & 1 & 1 & 13 & 32 & 5 & 28 \\
    pickup_truck & 7 & 6 & 15 & 16 & 12 & 14 & 28 & 2 \\
    keyboard & 5 & 13 & 9 & 46 & 17 & 4 & 0 & 6 \\
    lion & 0 & 3 & 0 & 2 & 1 & 94 & 0 & 0 \\
    clock & 1 & 2 & 15 & 15 & 15 & 41 & 8 & 3 \\
    trout & 30 & 10 & 4 & 10 & 2 & 28 & 4 & 12 \\
    orange & 0 & 0 & 0 & 0 & 0 & 98 & 2 & 0 \\
    woman & 0 & 0 & 0 & 36 & 49 & 14 & 0 & 1 \\
    shark & 8 & 24 & 29 & 20 & 8 & 7 & 1 & 3 \\
    sunflower & 1 & 0 & 0 & 1 & 0 & 96 & 2 & 0 \\
    pine_tree & 80 & 2 & 0 & 3 & 13 & 1 & 0 & 1 \\
    snake & 21 & 4 & 4 & 0 & 18 & 23 & 11 & 19 \\
    elephant & 0 & 73 & 0 & 1 & 25 & 1 & 0 & 0 \\
    possum & 0 & 20 & 3 & 10 & 6 & 58 & 0 & 3 \\
    \bottomrule
  \end{tabular}
  \end{adjustbox}
  \caption{\textbf{CIFAR100-F Statistics (part 2).} The number of instances that belongs to each foreground color from each class.}
  \label{tab:cifar100b_appendix}
\end{table*}
