# Supplementary material for: ColorSense: A Study on Color Vision in Machine Visual Recognition
Source: arXiv:2212.08650 source file (2025-02-13)
Supplement: Supplementary file 3 [file supp_fig_radar_cifar10_corruption.tex]

\begin{figure*}[h]
     \begin{subfigure}[b]{0.32\textwidth}
         \centering
         \includegraphics[width=\textwidth]{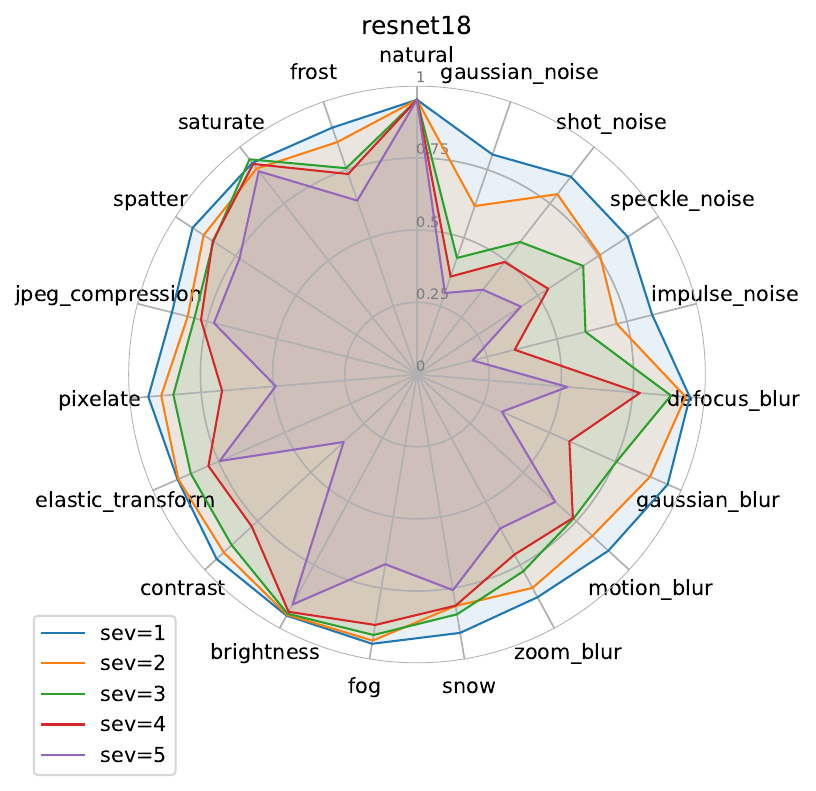}
        % \caption{}
     \end{subfigure}%\hfill
    %  \hspace{.9em}
     \begin{subfigure}[b]{0.32\textwidth}
         \centering
         \includegraphics[width=\textwidth]{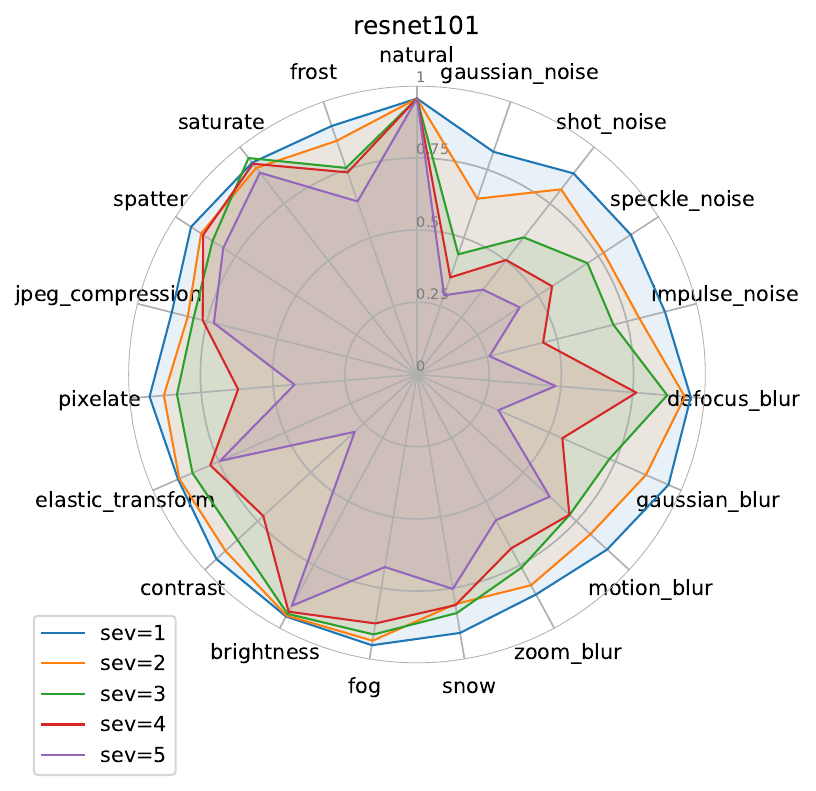}
        % \caption{}
     \end{subfigure}%\hfill
    %  \hspace{.9em}
     \begin{subfigure}[b]{0.32\textwidth}
         \centering
         \includegraphics[width=\textwidth]{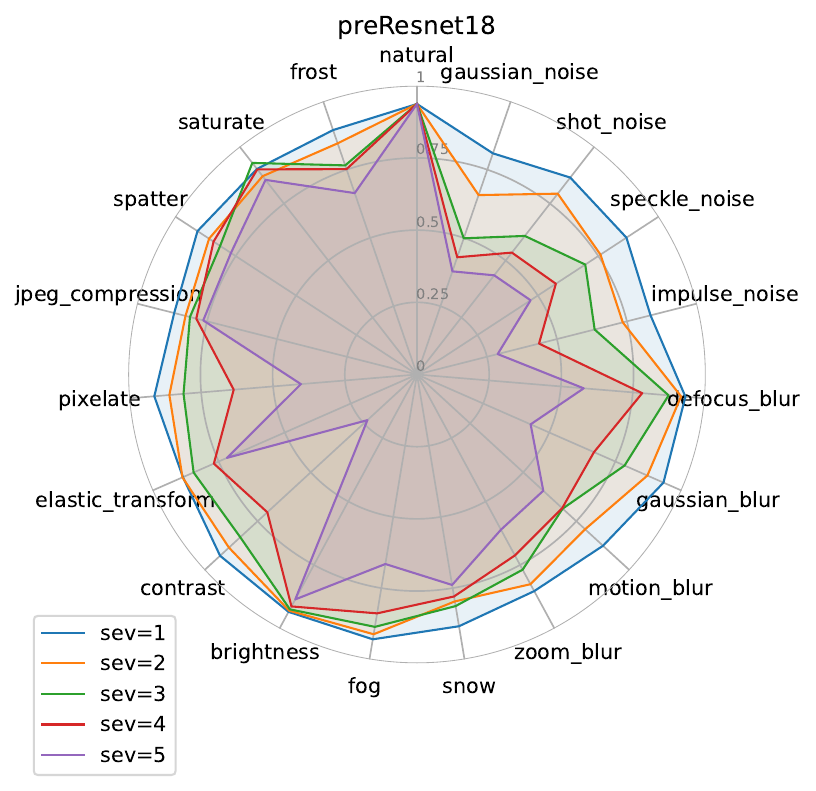}
        % \caption{}
     \end{subfigure}%\hfill
    %  \hspace{.9em}
    
     \begin{subfigure}[b]{0.32\textwidth}
         \centering
         \includegraphics[width=\textwidth]{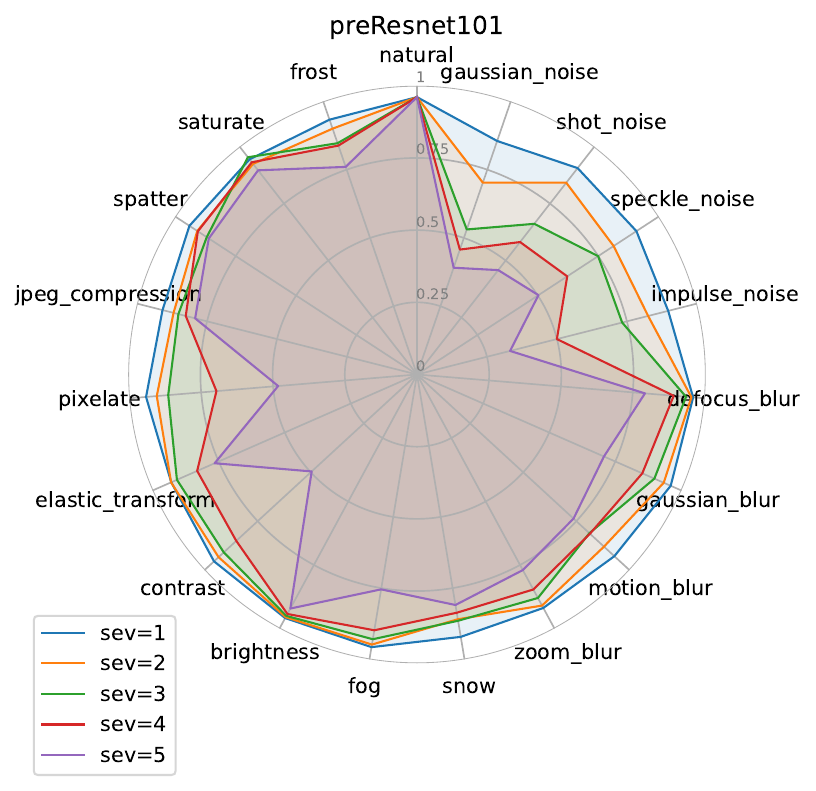}
        % \caption{}
     \end{subfigure}
     \begin{subfigure}[b]{0.32\textwidth}
         \centering
         \includegraphics[width=\textwidth]{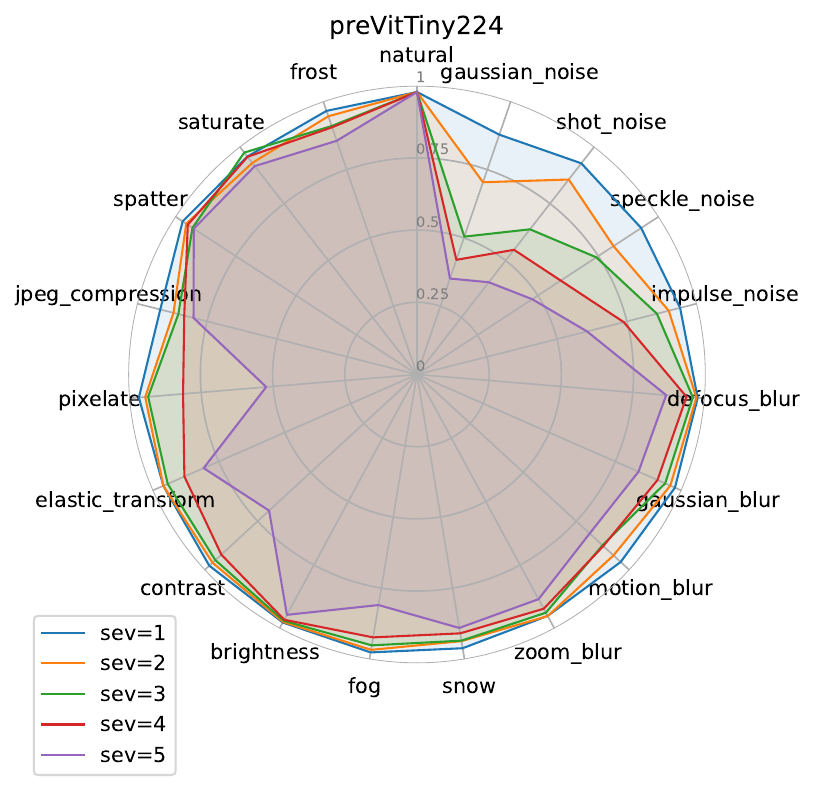}
        % \caption{}
     \end{subfigure}%\hfill
    %  \hspace{.9em}
     \begin{subfigure}[b]{0.32\textwidth}
         \centering
         \includegraphics[width=\textwidth]{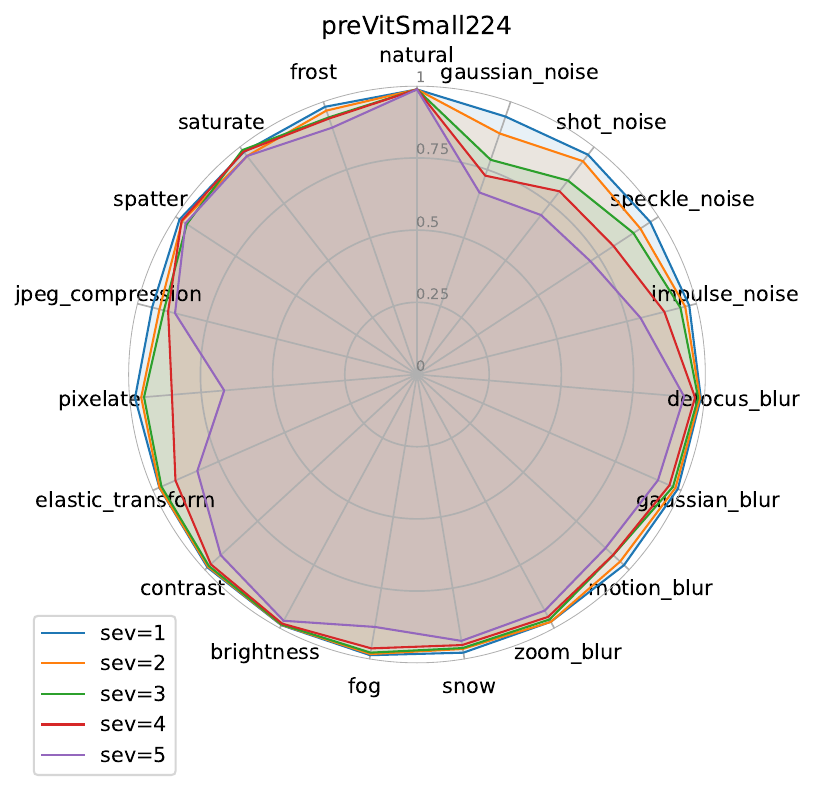}
        % \caption{}
     \end{subfigure}%\hfill
    %  \hspace{.9em}
    
     \caption{\textbf{Performance on each type of corruption in CIFAR10-C by severity.} The behavior on each level of severity and each type of corruption are different. We encourage joint further study on them with our CIFAR10-CoCo.}
     \label{fig:radar_cifar10c}
     \vspace{-3mm}
\end{figure*}
