# Supplementary material for: ColorSense: A Study on Color Vision in Machine Visual Recognition
Source: arXiv:2212.08650 source file (2025-02-13)
Supplement: Supplementary file 4 [file supp_tab_cifar10-f.tex]

\begin{table*}[h]
\centering
  \begin{adjustbox}{max width=\textwidth}
   \begin{tabular}{lcccccccc}
    \toprule
    Classes & Green & Gray & Blue & White & Black & Brown & Red & Others \\
     \midrule
    cat & 0 & 115 & 3 & 85 & 133 & 527 & 0 & 137 \\
    dog & 0 & 19 & 0 & 377 & 114 & 386 & 1 & 103 \\
    truck & 72 & 31 & 135 & 294 & 50 & 102 & 270 & 46 \\
    bird & 43 & 90 & 37 & 102 & 198 & 441 & 37 & 52 \\
    airplane & 108 & 150 & 138 & 298 & 152 & 86 & 45 & 23 \\
    ship & 39 & 61 & 117 & 429 & 98 & 87 & 110 & 59 \\
    frog & 420 & 69 & 8 & 6 & 29 & 396 & 23 & 49 \\
    horse & 6 & 21 & 7 & 288 & 142 & 510 & 3 & 23 \\
    deer & 6 & 46 & 3 & 29 & 75 & 834 & 0 & 7 \\
    automobile & 56 & 129 & 187 & 227 & 116 & 87 & 192 & 6 \\
    \bottomrule
  \end{tabular}
  \end{adjustbox}
  \caption{\textbf{CIFAR10-F Statistics.} The number of instances that belongs to each background color from each class.}
  \label{tab:cifar10f_appendix}
\end{table*}
